# Supplementary material for: Dynamic Graph Node Classification via Time Augmentation
Source: arXiv:2212.03449 source file (2022-12-07)
Supplement: Supplementary file 1 [file appendix.tex]

\appendix

\section{Hyper-parameter Settings}
\label{appendix:param}

In this section, we provide hyper-parameter setting details for \name~along with other baselines. For all models, we use Adam optimizer with learning rate of $0.01$ and weight decay of $0.0005$ for training. All models are trained for $200$ epochs, with a learning rate decay on plateau scheduler based on validation set macro-AUC performance. We use $128$ as node representation feature dimension. All models share the same MLP decoder architecture with dropout ratio $0.3$ to covert dynamic node representations to class logits.

For~\name, we use validation set performance to select time augmentation module type from three realizations.
We tune layer number from $\{2, 4, 8, 16, 32\}$, dropout ratio from $\{0.1, 0.3, 0.5\}$ and skip connection from $\{\mathrm{True}, \mathrm{False}\}$. $\lambda = l\cdot\beta_{l}$ from $\{0.5, 1.0, 1.5\}$ and $\alpha_l$ from $\{0.1, 0.3, 0.5\}$ are tuned following GCNII recommended suggestions using grid search. In addition, we also adopt GNCII variant, whose message passing mechanism is defined as
\begin{align}
\label{IPM_variant}
\mH^{l+1}=\sigma_{ip}\Big(&(1-\alpha_{l}) \hat{\mA} \mH^{l}\big((1-\beta_{l})\mI+\beta_{l}\mW_{1}^{l}\big) +\nonumber\\
&\alpha_{l} \mH^{0}\big((1-\beta_{l}) \mI+\beta_{l} \mW_{2}^{l}\big)\Big),
\end{align}
and select the better performing one as tuning variant from $\{\mathrm{True},$ $ \mathrm{False}\}$. Note that for the disentangled time-augmentation realization case, the layer number parameter is used for both structural graph $\mA_{s}$ and temporal graph $\mA_{t}$. 

We tune hyper-parameters of all baselines following their recommended suggestions. For GAT, we tune layer number from $\{2, 3, 4\}$, dropout ratio from $\{0.1, 0.3, 0.5\}$, attention head number from $\{4, 8, 16, 32\}$. Note that the layer number range is limited due to large memory requirement. For GCNII, we tune layer number from $\{2, 4, 8, 16, 32, 64\}$, dropout ratio from $\{0.1, 0.3, 0.5\}$, $\lambda = l\cdot\beta_{l}$ from $\{0.5, 1.0, 1.5\}$, $\alpha_l$ from $\{0.1, 0.3, 0.5\}$ and variant from $\{\mathrm{True}, \mathrm{False}\}$ following the paper's original hyper-parameter tuning guidelines.

Since both dynamic graph learning methods demonstrate large memory requirement, the layer number tuning range is limited. For EvolveGCN, we select the model type from EvolveGCN-H and EvolveGCN-O based on validation performance, while we tune layer number from $\{2, 3, 4\}$. For DySAT, we use $0.1$ and $0.5$ as spatio and temporal dropout ratio respectively as recommended, and we tune number of structural and temporal layers from $\{1, 2\}$ and number of structural and temporal heads from $\{8, 16\}$. 

\section{\name~for Disentangled Case}
\label{appendix:variants}
In this section, we describe~\name~'s architecture corresponding to the disentangled time-augmentation realization case as the time augmentation module.
After we define $\mA_{s}, \mA_{t}$ as the structural and temporal graph respectively, we first use one information propagation module for the structural graph $\mA_{s}$. 
After we obtain $\mH_s$ which summarizes structural information, we apply the second information propagation module guided by the temporal graph $\mA_{t}$, with $\mH_s$ as the initial node embedding input. 
Finally, we use $\mH_t$ that summarizes both structural and temporal dynamics for the dynamic node classification task.

\section{Efficiency Experiment}
\label{appendix:efficiency}
Figure~\ref{fig:efficiency} compares the average training time per epoch between \name~versus other dynamic baseline methods,~\ie, DySAT and EvolveGCN.
Figure's x-axis represents number of snapshots used for model training and the y-axis represents the average time spent per epoch at the corresponding time steps.
We use the green color to indicate~\name~and use blue and orange to indicate DySAT and EvolveGCN. 

% \section{Ablation Study}
% \label{appendix:ablation}
% \subsection{Experimental Setup}
% % % In addition to the lightweight convolution, ~\name's Temporal Sequence Learning module also consists several components. 
% % % We conduct this ablation study to analyze how each of the 
% % % We select four components that consist of the Temporal Sequence Learning module to analyze 
% % The four components we select to analyze in the Ablation Study as described in Sec.~\ref{rq3} are: 1) weighted softmax normalization in the lightweight convolution operator; 2) GLU; 3) feed-forward layer with ReLU activatio; and 4) residual connections.
% % We conduct an exhaustive search on all possible combination of different components to construct $2^4=16$ model variants and compare their performance in Table.~\ref{tab:ablation_macro} (macro-AUC) and Table.~\ref{tab:ablation_micro} (micro-AUC) where a~\cmark~symbol indicates the presence of the corresponding component and a~\xmark~symbol indicates its absence.
% % We select two datasets (\textit{Enron-I} and \textit{Radoslaw}) as they can be considered as dynamic graph representatives with different time step lengths.
% % Similar to the Link Prediction Experiments (Sec.~\ref{sec:rq1}), we use three different random seeds to train~\name~for $200$ epoches with a $512$ batch size.
% % The experiments were conducted using Nvidia Tesla P100 with 48 CPU cores.
